# Supplementary material for: Bridging GenAI policy and practice: Brief instruction improves learning-oriented prompting in an introductory programming course
Source: arXiv:2602.16033 source file (2026-11-12)
Supplement: Supplementary file 1 [file supplementary.tex]

\documentclass[10pt]{article}
\usepackage[margin=2.2cm]{geometry}
\usepackage{booktabs}
\usepackage{multirow}
\usepackage{array}
\usepackage{caption}
\usepackage{graphicx}
\usepackage[hidelinks]{hyperref}
\captionsetup{font=small,labelfont=bf,justification=raggedright,singlelinecheck=false}

% Supplementary tables and figures are numbered S1, S2, ...
\renewcommand{\thetable}{S\arabic{table}}
\renewcommand{\thefigure}{S\arabic{figure}}
\renewcommand{\tablename}{Supplementary Table}
\renewcommand{\figurename}{Supplementary Fig.}

\begin{document}

\title{Supplementary Information}
\author{}
\date{}
\maketitle

\input{supplementary_body}

\end{document}
